# Supplementary material for: Closed loop BCI System for Cybathlon 2020
Source: arXiv:2212.04172 source file (2023-02-02)
Supplement: Supplementary file 1 [file Supplementary_Materials.pdf]

# Supplementary Materials

## of Closed loop BCI System for Cybathlon 2020

Csaba Köllőd, *Member, IEEE*, András Adolf, *Member, IEEE*, Gergely Márton, *Fellow, IEEE*, Moutz Wahdow, *Member, IEEE*, Ward Fadel, *Member, IEEE* and István Ulbert, *Fellow, IEEE*

### I. General Offline Paradigm

We designed a general-purpose paradigm execution framework code named a General Offline Paradigm (GoPar) controlling program. This program can be found at https://github.com/kolcs/GoPar. With the aid of this code, different MI paradigms could be executed by giving visual instructions to subjects concerning the selected paradigm and registering all the trigger events which were displayed on a monitor. The events were synchronized with the raw EEG signals. GoPar was developed so that both abled and disabled subjects could also use it, executing MI tasks overtly or covertly only relevant to abled subjects. This code aims to record a high number of labeled data that can be used to train the classifier part of the BCI system. The GoPar was custom written in MATLAB using the Psychophysics Toolbox extension [1], [2]. With the aid of the GoPar program, 4 active (overt or covert) motor movement tasks were carried out, called Task1, Task2, Task3, and Task4 types, and one inactive task, with an idle period between them, called the Rest task. With the aid of the GoPar code, many different MI paradigms can be created by defining concrete motor movement types (body parts to move overtly or covertly) for each task type (Task1, Task2, Task3, and Task4).

Before an experiment, subjects were asked to avoid blinking, swallowing, clenching, or any movements or facial expression unrelated to the actual task during the task periods and try to execute only the required motor movements repeatedly while the fixation cross was present. During the rest period, the paradigm control program presented the next task on the screen in written form. During this period, subjects were allowed to blink, swallow, and execute any movement. Subjects were instructed to perform the motor tasks for 4 seconds and the rest task for 3 seconds.

The GoPar experimental session, presented in Figure 1, started with a one-minute-long period when the subject was required to open his eyes and focus on the cross presented on the screen. This session was followed by the instruction of a one-minute-long closed-eye period. In both cases, the subject had to sit as calmly as possible, physically and mentally, without any thoughts. 2 warmup sessions followed the eyes-open and eyes-closed period.

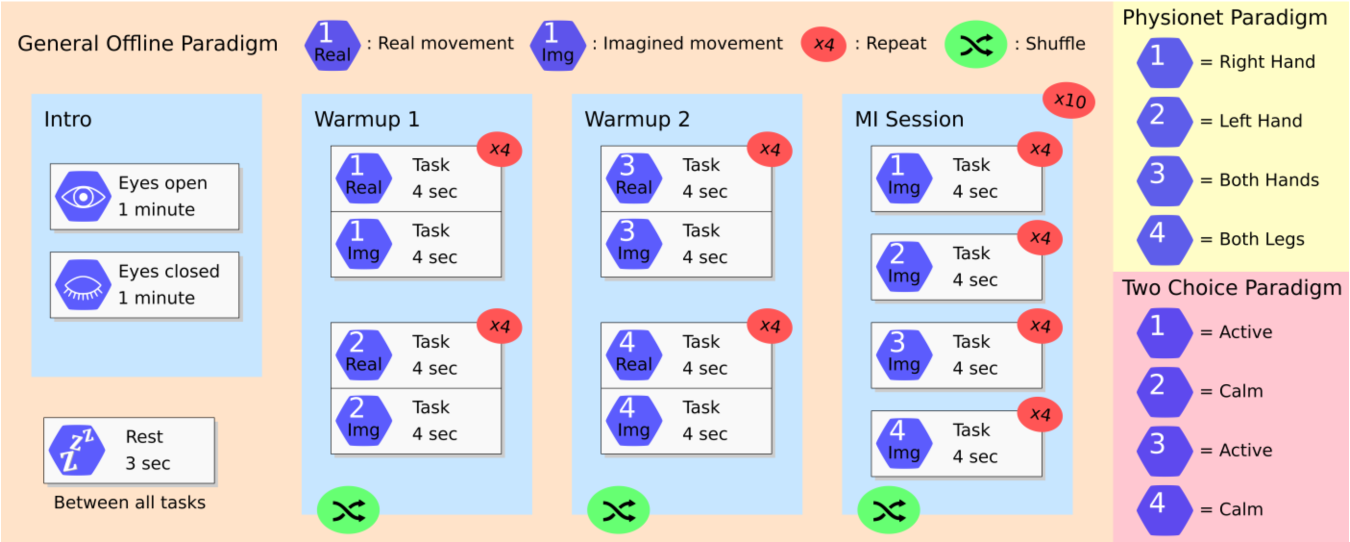

1. Figure - General Offline Paradigm (GoPar): The paradigm execution framework code of GoPar, was designed to lead different motor imaginary (MI) based paradigms with 4 types of MI movements for both abled and disabled subjects. All tasks are separated with a 3-second long resting period. A specific paradigm can be conducted by defining concrete MI tasks. The GoPar starts with an introduction session, where 1-minute-long eyes open and 1-minute-long eyes closed tasks are required. Then, it is followed by two warmup sessions, where the MI movements are practiced. In each warmup session, 2 tasks are selected and presented four times to the experimental subject in a randomized order. For each task, first, a 4-second long overt movement is required, followed by a 4-second long covert movement. These warmup sessions can be excluded for disabled subjects. The GoPar concludes with 10 MI sessions. In one MI session, 4-second-long MI tasks are required. Each task is repeated four times, and the order of the task is randomized. Our Two Choice Paradigm can be conducted by indicating the assignment in the figure's bottom right corner.

In the first warmup session, Task1 and Task2 were selected. For each task type (e.g., Task 1), first, an executed, overt motor movement was required with the instructed limb, which was followed by a Rest period and continuing with the imagined execution of the same limb as before the Rest period. Then a new task type was selected (e.g., Task 2), and the previous procedure was repeated. One task was presented 8 times during one session, including the overt and covert executions, and the order of Task1 and Task2 were randomized. In the second warmup session, Task3 and Task4 were selected and instructed to move overtly and covertly. These sessions were excluded for our pilots.

After the two warmup sessions, the experiment was followed by 10 additional sessions. These MI sessions contained only imagined covert motor movements. Each task was presented 4 times in one session, and the order of the task types was randomized. After each completed session, the subjects were allowed to take a break with a self-defined length without leaving the experimental setup.

The Physionet paradigm could have been easily copied by assigning MI tasks for the four task types in GoPar as follows:

- Task1 – Right-hand movement
- Task2 – Left-hand movement
- Task3 – Both hand movements
- Task4 – Both leg movements

The Two Choice Paradigm was defined in GoPar with the following assignment:

- Task1 and Task3 – Active MI task
- Task2 and Task4 – Calm task

## References

[1] D. H. Brainard, “The Psychophysics Toolbox,” *Spat. Vis.*, vol. 10, no. 4, pp. 433–436, Jan. 1997, doi: 10/c7g6rj.

[2] M. Kleiner, D. Brainard, and D. Pelli, “What’s new in Psychtoolbox-3?,” *Percept. 36 ECVP Abstr. Suppl.*, 2007.
